# Supplementary material for: Is Repeated Bayesian Interim Analysis Consequence-Free?
Source: arXiv:2508.07403 source file (2025-12-28)
Supplement: Supplementary file 1 [file supplementary_v10.tex]

\documentclass[12pt]{article}
\usepackage{setspace}
\usepackage{mathrsfs}
\usepackage{amsmath,verbatim, latexsym, amssymb,epsfig,lscape}
\usepackage{graphicx,setspace,float,longtable}
\usepackage{cite}

\setlength{\topmargin}{-0.2in} \setlength{\oddsidemargin}{0.05 in}
\setlength{\textwidth}{6.5in} \setlength{\textheight}{8.5in}
\usepackage[dvipsnames,usenames]{color}         %for colors

  \pdfminorversion=4 
  
\begin{document}
\begin{center}
{\Large \bf Supplementary Materials for ``Is Repeated Bayesian Interim Analysis Consequence-Free?"}
\end{center}

\begin{center}
	Suyu Liu$^1$, Beibei Guo$^2$,  Laura Thompson$^3$, Lei Nie$^3$, Ying Yuan$^{2, *}$,\\
\end{center}
\noindent{
$^1$Department of Biostatistics, The University of Texas MD Anderson Cancer Center, Houston, TX\\
$^2$Department of Experimental Statistics, Louisiana State University, Baton Rouge, LA 70803, USA \\
$^3$ Center for Drug Evaluation and Research, Food and Drug Administration (FDA), Silver Spring, MD\\
$^*$ Email: yyuan@mdanderson.org

\setcounter{table}{0}
\renewcommand{\thetable}{S\arabic{table}}

\setcounter{figure}{0}
\renewcommand{\thefigure}{S\arabic{figure}}

\doublespacing

%% Setting up the document class and necessary packages
%\documentclass[a4paper,11pt]{article}
%\usepackage{amsmath, amssymb, amsthm}
%\usepackage{geometry}
%\geometry{margin=1in}
%\usepackage{enumitem}
%\usepackage{mathrsfs}
%
%% Defining theorem environments
%\theoremstyle{plain}
%\newtheorem{theorem}{Theorem}
%\newtheorem{lemma}{Lemma}
%\newtheorem{definition}{Definition}

% Configuring font (using standard LaTeX fonts for PDFLaTeX compatibility)
%\usepackage{times}

% Title and section
\bigskip \bigskip
%\subsection*{1. Proof of FDR Inflation in Adaptive Design with Interim Analyses for Superiority Stopping}

\subsection*{Proof of FDR and pFDR Inflation under Sequential Monitoring}

Let $\theta \in \Theta$ represent the parameter of interest, and define two disjoint states of nature: the ineffective state $S_0 = \{\theta : \theta \le \theta_0\}$ and the effective state $S_1 = \{\theta : \theta > \theta_0\}$. Under the data-generating prior $\pi_g(\theta)$, the prior probability that a treatment is ineffective is $w_0 = \int_{S_0} \pi_g(\theta) d\theta$. 

For a single trial, let $R \in \{0, 1\}$ be the indicator that the treatment is declared effective, and $V = \mathbb{I}(R=1 \text{ and } \theta \in S_0)$ be the indicator of a false claim. Based on the definition of the positive False Discovery Rate, we have:
\begin{equation}
\text{pFDR} = \mathbb{E}\left[\frac{V}{R} \mid R>0 \right] = \Pr(S_0 \mid R=1) = \frac{w_0 \alpha}{w_0 \alpha + (1-w_0) \gamma},
\end{equation}
where $\alpha = \Pr(R=1 \mid S_0)$ and $\gamma = \Pr(R=1 \mid S_1)$. 

Consider a fixed design with a single analysis at sample size $N$ using the claim indicator $R_F = \mathbb{I}(q_N > C)$, where $q_n = \Pr(\theta \in S_1 \mid \mathcal{D}_n)$ is the posterior probability of effectiveness. In contrast, an adaptive design with $K$ looks at $n_1, \dots, n_K = N$ employs the indicator $R_A = \mathbb{I}(\max_{k \le K} q_{n_k} > C)$. By the monotonicity of probability measures and the fact that $\{q_N > C\} \subseteq \{\max_{k \le K} q_{n_k} > C\}$, it holds that $\alpha_A \ge \alpha_F$ and $\gamma_A \ge \gamma_F$.

The pFDR is a strictly increasing function of the ratio $\rho = \alpha / \gamma$. To demonstrate that $\text{pFDR}_A > \text{pFDR}_F$, it is sufficient to show that $\rho_A > \rho_F$, which is equivalent to:
\begin{equation}
\label{eq:ratio_inflation}
\frac{\alpha_A}{\alpha_F} > \frac{\gamma_A}{\gamma_F}.
\end{equation}

Under the matched-prior assumption, the sequence of posterior probabilities $\{q_{n_k}\}_{k=1}^K$ is a martingale with respect to the filtration $\mathcal{F}_{n_k}$. Under state $S_0$, the probability of the running maximum exceeding $C$ ($\alpha_A$) accumulates significantly more mass than the terminal value $q_N$ ($\alpha_F$) due to the stochastic fluctuations of the martingale over multiple looks.

Furthermore, while both $\alpha$ and $\gamma$ increase in the adaptive setting, $\gamma$ is bounded above by $1$. Clinical designs are typically powered such that $\gamma_F$ is already high (e.g., $0.8$ or $0.9$), meaning the relative increase $\gamma_A / \gamma_F$ is mathematically constrained. Conversely, $\alpha_F$ is usually small, allowing for a much larger relative increase in $\alpha$ as $K$ increases. Thus, the condition in \eqref{eq:ratio_inflation} holds, and $\text{pFDR}_A > \text{pFDR}_F$.

To extend this to the original FDR, we utilize the relationship $\text{FDR} = \text{pFDR} \cdot \Pr(R > 0)$. Since the adaptive design makes a discovery whenever the fixed design does, $\Pr(R_A > 0) \ge \Pr(R_F > 0)$. Given that $\text{pFDR}_A > \text{pFDR}_F$ and $\Pr(R_A > 0) \ge \Pr(R_F > 0)$, it follows that:
\begin{equation}
\text{FDR}_A = \text{pFDR}_A \cdot \Pr(R_A > 0) > \text{pFDR}_F \cdot \Pr(R_F > 0) = \text{FDR}_F.
\end{equation}
Therefore, sequential Bayesian monitoring with superiority stopping rules results in the inflation of both FDR and pFDR relative to a fixed-sample design.

\newpage
\subsection*{2. Simulation parameters for RCTs}
For both binary and normal outcomes, the data-generating prior $\pi_g(\theta)$ and user-specified prior $\pi(\theta)$ for the treatment arm were set to match those used in the single-arm trial simulations. The equivalence margin $\delta=0$. The parameter specifications for the control arm and probability cutoff $C$ are detailed below.

For the binary outcome, the data-generating prior for the standard treatment efficacy $\theta_0$ was specified as $\pi_g(\theta_0)=$ Beta(359.4, 239.6), and the user-specified prior was $\pi(\theta_0)=\mbox{Beta}(36,24)$. The cutoff $C=0.82$. For the normal outcome with a known variance of 1, $\pi_g(\theta_0)=$ Normal(0.25, 0.0009), and $\pi(\theta_0) =\mbox{Normal}(0.25,0.01)$. The cutoff $C=0.55$. For the normal outcome with an unknown variance, $\pi_g(\theta_0)=N(0.25,0.0009)$, and the true variance for the control arm was set to 40. The user-specified prior for the control arm was $\pi(\theta_0|\sigma_0^2)=N(0.25,\sigma_0^2/100)$ and $\pi(\sigma_0^2)=\mbox{Inv-}\chi^2(100,40)$. The cutoff $C=0.72$. Tables S1, S2, and S3 report the design metrics for these three outcome types.

For RCTs with time-to-event outcomes, we set  $\rho=1$, assuming the following data-generating priors: $\pi_g(\theta)=\mbox{Gamma}(12,2)$, $\pi_g(\kappa)=\mbox{Gamma}(8,2)$, and $\pi_g(\beta)= N(0,1)$. The cutoff $C=0.57$. The corresponding results are presented in Table S4.

\clearpage
\subsection*{3. Additional Simulation Results}

\begin{table}[h]
\begin{center}
\begin{footnotesize}
\caption{RCT with binary outcomes: pFDR, FDR, bias, MSE,  coverage of posterior credible intervals, and ATIE, evaluated with or without interim stopping, under various user-specified priors. Data-generating prior is $\pi_g(\theta) = \mbox{Beta}(3,3)$. }
\begin{tabular}{lcccccccccc}
\hline
\hline

$\pi(\theta)$ &      Interims &        pFDR &     FDR &     Bias  ($\times 10^{-3}$)                    &    MSE & Coverage &      ATIE     \\

 %                 &                    &                   &            &   ($\times 10^{-3}$)    &            &         &           \\
\hline

Beta(18, 12) &         no &      0.049&0.009&36.984&0.008&0.727&0.013 \\

           &        yes &      0.078&0.016&33.988&0.009&0.718&0.023\\

      &            &            &            &            &            &            &                   \\
      
Beta(3.6, 2.4) &         no &      0.058&0.012&10.515&0.004&0.946&0.018 \\

           &        yes &      0.107&0.027&12.995&0.005&0.946&0.039 \\

            &            &            &            &            &            &            &                   \\

Beta(0.06, 0.04) &         no &      0.062&0.014&0.125&0.004&0.946&0.020\\

           &        yes &      0.121&0.032&8.818&0.006&0.937&0.047 \\

            &            &            &            &            &            &            &                   \\

Beta(15, 15) &         no &      0.017&0.002&-0.516&0.007&0.763&0.003 \\

           &        yes &      0.023&0.003&-2.686&0.007&0.758&0.004 \\

            &            &            &            &            &            &            &                   \\

Beta(3, 3) &         no &      0.044&0.008&-0.199&0.004&0.950&0.012 \\

           &        yes &      0.080&0.018&-0.089&0.004&0.949&0.026 \\

            &            &            &            &            &            &            &                   \\

Beta(0.05, 0.05) &         no &      0.062&0.014&-0.074&0.004&0.946&0.020 \\

           &        yes &      0.119&0.031&8.467&0.006&0.937&0.046 \\

            &            &            &            &            &            &            &                   \\

Beta(21, 9) &         no &      0.117&0.031&74.484&0.012&0.623&0.046 \\

           &        yes &      0.223&0.076&77.508&0.014&0.609&0.111 \\

            &            &            &            &            &            &            &                   \\

Beta(4.2, 1.8) &         no &    0.075&0.017&21.230&0.004&0.936&0.026 \\

           &        yes &      0.139&0.039&26.864&0.006&0.932&0.057  \\

            &            &            &            &            &            &            &                   \\

Beta(0.07, 0.03) &         no &     0.062&0.014&0.325&0.004&0.946&0.020  \\

           &        yes &     0.121&0.032&9.080&0.006&0.937&0.047 \\

\hline
\hline
\end{tabular}
\end{footnotesize}
\end{center}
\end{table}

\begin{table}
\begin{center}
\begin{footnotesize}
\caption{RCT with normal outcomes with a known variance of 1: pFDR, FDR, bias, MSE,  coverage of posterior credible intervals, and ATIE,  evaluated with or without interim stopping, under various user-specified priors. Data-generating prior is $\pi_g(\theta) = \mbox{Normal}(0,1)$. }
\begin{tabular}{lccccccc}
\hline
\hline

$\pi(\theta)$ &      Interims &        pFDR &     FDR &     Bias  ($\times 10^{-3}$)                    &    MSE & Coverage &      ATIE     \\

 %                 &                    &                   &            &   ($\times 10^{-3}$)    &            &         &           \\
\hline

N(0.25, 0.2) &         no &      0.051&0.020&22.881&0.026&0.900&0.034\\

           &        yes &     0.097&0.041&0.956&0.042&0.885&0.069 \\

              &            &            &            &            &            &            &                   \\

N(0.25, 1) &         no &      0.051&0.020&4.908&0.020&0.949&0.034 \\

           &        yes &      0.097&0.041&7.772&0.031&0.949&0.069\\

              &            &            &            &            &            &            &                   \\

N(0.25, 1000) &         no &      0.051&0.020&-0.030&0.020&0.948&0.034 \\

           &        yes &      0.097&0.041&11.338&0.033&0.948&0.069 \\

               &            &            &            &            &            &            &                   \\

 N(0, 0.2) &         no &      0.043&0.017&0.154&0.025&0.905&0.028 \\

           &        yes &      0.075&0.031&-32.296&0.045&0.882&0.051\\

                 &            &            &            &            &            &            &                   \\

   N(0, 1) &         no &     0.050&0.020&0.006&0.020&0.949&0.033 \\

           &        yes &      0.093&0.039&0.087&0.031&0.950&0.066 \\

                   &            &            &            &            &            &            &                   \\

N(0, 1000) &         no &      0.051&0.020&-0.035&0.020&0.948&0.034\\

           &        yes &      0.097&0.041&11.330&0.033&0.948&0.069 \\

                    &            &            &            &            &            &            &                   \\

N(0.5, 0.2) &         no &      0.062&0.025&45.609&0.027&0.889&0.042 \\

           &        yes &      0.120&0.053&35.374&0.042&0.879&0.089\\
           
         &            &            &            &            &            &            &                   \\

 N(0.5, 1) &         no &      0.053&0.021&9.810&0.020&0.948&0.035 \\

           &        yes &     0.102&0.044&15.553&0.032&0.949&0.073 \\

                    &            &            &            &            &            &            &                   \\

N(0.5, 1000) &         no &     0.051&0.020&-0.025&0.020&0.948&0.034 \\

           &        yes &     0.097&0.041&11.346&0.033&0.948&0.069\\

\hline
\hline
\end{tabular}
\end{footnotesize}
\end{center}
\end{table}

\begin{table}
\begin{center}
\begin{footnotesize}
\caption{RCT with normal outcomes with an unknown variance: pFDR, FDR, bias, MSE,  coverage of posterior credible intervals, and ATIE,  evaluated with or without interim stopping, under various user-specified priors. Data-generating prior is $\pi_g(\theta|\sigma^2)= N(0,\sigma^2/5)$ and $\pi_g(\sigma^2)= \mbox{Inv-}\chi^2(5,40)$.}
\begin{tabular}{lccccccc}
\hline
\hline

$\pi(\theta)$ &      Interims &        pFDR &     FDR &     Bias  ($\times 10^{-3}$)                    &    MSE & Coverage &      ATIE     \\

 %                 &                    &                   &            &   ($\times 10^{-3}$)    &            &         &           \\
\hline

$\theta|\sigma^2\sim N(0.25,\sigma^2/20)$ &         no &      0.049&0.018&69.812&1.781&0.857&0.034 \\

$\sigma^2\sim Inv-\chi^2(20,40)$ &        yes &      0.086&0.036&-90.409&2.696&0.832&0.068 \\

           &            &            &            &            &            &            &                   \\

$\theta|\sigma^2\sim N(0.25,\sigma^2/5)$ &         no &      0.052&0.020&23.931&1.229&0.950&0.038 \\

$\sigma^2\sim Inv-\chi^2(5,40)$ &        yes &     0.099&0.043&36.395&1.776&0.951&0.081 \\

          &            &            &            &            &            &            &                   \\

$\theta|\sigma^2\sim N(0.25,\sigma^2/0.1)$ &         no &      0.053&0.021&2.991&1.344&0.948&0.039 \\

$\sigma^2\sim Inv-\chi^2(0.1,40)$ &        yes &      0.105&0.047&175.694&2.177&0.946&0.088 \\

           &            &            &            &            &            &            &                   \\

$\theta|\sigma^2\sim N(0,\sigma^2/20)$ &         no &      0.043&0.015&-1.617&1.776&0.857&0.029 \\

$\sigma^2\sim Inv-\chi^2(20,40)$ &        yes &      0.073&0.029&-174.562&2.726&0.831&0.055 \\

           &            &            &            &            &            &            &                   \\

$\theta|\sigma^2\sim N(0,\sigma^2/5)$ &         no &      0.050&0.019&1.204&1.228&0.950&0.036 \\

$\sigma^2\sim Inv-\chi^2(5,40)$ &        yes &      0.095&0.041&3.478&1.766&0.951&0.077\\

          &            &            &            &            &            &            &                   \\

$\theta|\sigma^2\sim N(0,\sigma^2/0.1)$ &         no &     0.053&0.021&2.492&1.344&0.948&0.039 \\

$\sigma^2\sim Inv-\chi^2(0.1,40)$ &        yes &      0.105&0.047&174.951&2.176&0.946&0.088\\

          &            &            &            &            &            &            &                   \\

$\theta|\sigma^2\sim N(0.5,\sigma^2/20)$ &         no &      0.055&0.021&141.240&1.796&0.855&0.040 \\

$\sigma^2\sim Inv-\chi^2(20,40)$ &        yes &     0.101&0.044&-2.570&2.681&0.832&0.083 \\

          &            &            &            &            &            &            &                   \\

$\theta|\sigma^2\sim N(0.5,\sigma^2/5)$ &         no &      0.053&0.021&46.659&1.230&0.950&0.039\\

$\sigma^2\sim Inv-\chi^2(5,40)$ &        yes &     0.103&0.045&69.378&1.788&0.950&0.085 \\

          &            &            &            &            &            &            &                   \\

$\theta|\sigma^2\sim N(0.5,\sigma^2/0.1)$ &         no &      0.053&0.021&3.490&1.344&0.948&0.039 \\

$\sigma^2\sim Inv-\chi^2(0.1,40)$ &        yes &      0.105&0.047&176.562&2.178&0.946&0.088\\

\hline
\hline

\end{tabular}
\end{footnotesize}
\end{center}
\end{table}

\begin{table}
\begin{center}
\begin{footnotesize}
\caption{RCT with survival outcomes:  pFDR, FDR, bias, MSE,  coverage of posterior credible intervals, and ATIE, evaluated with or without interim stopping, under various user-specified priors.  $\rho=1$, and data-generating prior is $\pi_g(\theta)=\mbox{Gamma}(12,2)$, $\pi_g(\kappa)=\mbox{Gamma}(8,2)$, and $\pi_g(\beta)=N(0,1)$.}
\begin{tabular}{lccccccc}
\hline
\hline

$\pi(\theta)$ &      Interims &        pFDR &     FDR &     Bias  ($\times 10^{-3}$)                    &    MSE & Coverage &      ATIE     \\

 %                 &                    &                   &            &   ($\times 10^{-3}$)    &            &         &           \\
\hline

$\theta\sim\mbox{Gamma}(72,12)$ &         no &      0.058&0.028&-227.114&1.302&0.823&0.056 \\

$\kappa\sim\mbox{Gamma}(32,8)$ &        yes &      0.175&0.100&-163.849&1.428&0.736&0.200 \\

$\beta\sim N(0, 0.2)$ &            &            &            &            &            &            &                 \\

                                  &            &            &            &            &            &            &                   \\
           
$\theta\sim\mbox{Gamma}(12, 2)$ &         no &      0.055&0.027&-0.168&0.476&0.941&0.054 \\

$\kappa\sim\mbox{Gamma}(8, 2)$ &        yes &      0.177&0.103&-0.023&0.576&0.937&0.207 \\

$\beta\sim N(0, 1)$ &            &            &            &            &            &            &                 \\

                                  &            &            &            &            &            &            &                   \\

$\theta\sim\mbox{Gamma}(0.36, 0.06)$ &         no &      0.056&0.027&117.396&0.877&0.938&0.054 \\

$\kappa\sim\mbox{Gamma}(0.16, 0.04)$ &        yes &      0.176&0.103&57.058&1.617&0.880&0.205 \\

$\beta\sim N(0, 100)$ &            &            &            &            &            &            &                 \\

                                  &            &            &            &            &            &            &                   \\

$\theta\sim\mbox{Gamma}(72,12)$ &         no &    0.037&0.017&-114.387&1.080&0.803&0.034 \\

$\kappa\sim\mbox{Gamma}(32,8)$ &        yes &      0.074&0.036&-33.551&1.137&0.728&0.071 \\

$\beta\sim N(0.405, 0.2)$ &            &            &            &            &            &            &                 \\

                                  &            &            &            &            &            &            &                   \\

$\theta\sim\mbox{Gamma}(12, 2)$ &         no &     0.050&0.024&33.334&0.482&0.940&0.049 \\

$\kappa\sim\mbox{Gamma}(8, 2)$ &        yes &      0.143&0.079&70.381&0.552&0.933&0.158\\

$\beta\sim N(0.405, 1)$ &            &            &            &            &            &            &                 \\

                                  &            &            &            &            &            &            &                   \\

$\theta\sim\mbox{Gamma}(0.36, 0.06)$ &         no &     0.056&0.027&117.756&0.900&0.940&0.055 \\

$\kappa\sim\mbox{Gamma}(0.16, 0.04)$ &        yes &      0.177&0.103&51.562&1.162&0.881&0.206 \\

$\beta\sim N(0.405, 100)$ &            &            &            &            &            &            &                 \\

                                  &            &            &            &            &            &            &                   \\

$\theta\sim\mbox{Gamma}(72,12)$ &         no &      0.107&0.057&-401.139&1.758&0.787&0.115\\

$\kappa\sim\mbox{Gamma}(32, 8)$ &        yes &      0.364&0.284&-585.687&2.409&0.661&0.568\\

$\beta\sim N(-0.693, 0.2)$ &            &            &            &            &            &            &                 \\

                                  &            &            &            &            &            &            &                   \\

$\theta\sim\mbox{Gamma}(12, 2)$ &         no &      0.064&0.032&-55.741&0.492&0.938&0.064 \\

$\kappa\sim\mbox{Gamma}(8, 2)$ &        yes &      0.241&0.155&-149.107&0.700&0.925&0.310 \\

$\beta\sim N(-0.693, 1)$ &            &            &            &            &            &            &                 \\

                                  &            &            &            &            &            &            &                   \\

$\theta\sim\mbox{Gamma}(0.36, 0.06)$ &         no &      0.056&0.027&116.109&0.859&0.939&0.054 \\

$\kappa\sim\mbox{Gamma}(0.16, 0.04)$ &        yes &     0.178&0.104&57.025&3.050&0.877&0.208 \\

$\beta\sim N(-0.693, 100)$ &            &            &            &            &            &            &                 \\

\hline
\hline
\end{tabular}
\end{footnotesize}
\end{center}
\end{table}

\begin{table}
\begin{center}
\begin{footnotesize}
\caption{Single-arm trials with binary outcomes under a fully sequential design: pFDR, FDR, bias, MSE,  coverage of posterior credible intervals, and ATIE, evaluated with or without interim stopping, under various user-specified priors with $\theta_0=0.6$ and data-generating prior $\pi_g(\theta) = \mbox{Beta}(3,3)$. }
\begin{tabular}{lccccccc}
\hline
\hline

$\pi(\theta)$ &      Interims &        pFDR &     FDR &     Bias  ($\times 10^{-3}$)                    &    MSE & Coverage &      ATIE     \\

%                  &                    &                   &            &   ($\times 10^{-3}$)    &            &          &           \\
\hline

Beta(18, 12) &         no &    0.060&0.017&22.970&0.004&0.793&0.025 \\

           &        yes &     0.200&0.073&16.466&0.006&0.764&0.107\\

           &            &            &            &            &            &            &                   \\

Beta(3.6, 2.4) &         no &   0.060&0.017&5.432&0.002&0.949&0.025 \\

           &        yes &      0.226&0.086&11.699&0.004&0.947&0.126 \\

          &            &            &            &            &            &            &                   \\

Beta(0.06, 0.04) &         no &      0.060&0.017&-0.167&0.002&0.948&0.025\\

           &        yes &     0.248&0.098&15.941&0.005&0.938&0.143 \\
           
          &            &            &            &            &            &            &                   \\

Beta(15, 15) &         no &    0.024&0.006&-0.107&0.003&0.822&0.008 \\

           &        yes &   0.063&0.017&-12.891&0.006&0.786&0.024 \\

              &            &            &            &            &            &            &                   \\

Beta(3, 3) &         no &     0.046&0.012&-0.228&0.002&0.950&0.018\\

           &        yes &     0.193&0.069&0.229&0.004&0.950&0.101\\

                &            &            &            &            &            &            &                   \\

Beta(0.05, 0.05) &         no &  0.060&0.017&-0.267&0.002&0.948&0.025 \\

           &        yes &     0.248&0.098&15.703&0.005&0.938&0.143\\

                &            &            &            &            &            &            &                   \\

Beta(21, 9) &         no &   0.122&0.040&46.047&0.005&0.713&0.059 \\

           &        yes &    0.404&0.211&63.101&0.010&0.652&0.309 \\

                     &            &            &            &            &            &            &                   \\

Beta(4.2, 1.8) &         no &    0.079&0.023&11.093&0.002&0.943&0.034 \\

           &        yes &   0.269&0.111&24.562&0.005&0.933&0.162\\

                     &            &            &            &            &            &            &                   \\
                     
Beta(0.07, 0.03) &         no &     0.060&0.017&-0.067&0.002&0.948&0.025\\

           &        yes &     0.248&0.098&16.177&0.005&0.937&0.144\\

\hline
\hline
\end{tabular}
\end{footnotesize}
\end{center}
\end{table}

\begin{table}
\begin{center}
\begin{footnotesize}
\caption{Single-arm trials with normal outcomes with a known variance of 1 under a fully sequential design: pFDR, FDR, bias, MSE,  coverage of posterior credible intervals, and ATIE, evaluated with or without interim stopping, under various user-specified priors with $\theta_0=0.25$ and data-generating prior $\pi_g(\theta) = N(0,1)$. }
\begin{tabular}{lccccccc}
\hline
\hline

$\pi(\theta)$ &      Interims &        pFDR &     FDR &     Bias  ($\times 10^{-3}$)                       &    MSE & Coverage &       ATIE     \\

    %              &                    &                   &            &   ($\times 10^{-3}$)    &            &    Rate      &     Rate      \\
\hline

N(0.25, 0.2) &         no &      0.051&0.021&12.176&0.012&0.925&0.035 \\

           &        yes &      0.162&0.077&-17.976&0.036&0.902&0.129 \\

                  &            &            &            &            &            &            &                   \\

N(0.25, 1) &         no &    0.051&0.021&2.660&0.010&0.949&0.035 \\

           &        yes &     0.160&0.076&6.967&0.027&0.949&0.127 \\

                      &            &            &            &            &            &            &                   \\

N(0.25, 1000) &         no &      0.051&0.021&0.165&0.010&0.950&0.035 \\

           &        yes &      0.160&0.076&15.790&0.029&0.949&0.127 \\

                &            &            &            &            &            &            &                   \\

 N(0, 0.2) &         no &     0.045&0.018&0.271&0.011&0.927&0.030 \\

           &        yes &      0.139&0.064&-46.905&0.040&0.892&0.107 \\

                     &            &            &            &            &            &            &                   \\

   N(0, 1) &         no &      0.050&0.020&0.185&0.010&0.950&0.034 \\

           &        yes &    0.156&0.074&0.264&0.027&0.950&0.123 \\

                &            &            &            &            &            &            &                   \\

N(0, 1000) &         no &     0.051&0.021&0.163&0.010&0.950&0.035 \\

           &        yes &    0.160&0.076&15.783&0.029&0.949&0.127\\

                  &            &            &            &            &            &            &                   \\

N(0.5, 0.2) &         no &     0.058&0.024&24.081&0.012&0.919&0.040 \\

           &        yes &     0.187&0.092&12.645&0.034&0.902&0.154 \\

                  &            &            &            &            &            &            &                   \\

 N(0.5, 1) &         no &    0.053&0.022&5.136&0.010&0.949&0.036\\

           &        yes &       0.166&0.079&13.850&0.028&0.949&0.132 \\

                   &            &            &            &            &            &            &                   \\

N(0.5, 1000) &         no &      0.051&0.021&0.168&0.010&0.950&0.035 \\

           &        yes & 0.160&0.076&15.797&0.029&0.949&0.127 \\
           
\hline
\hline
\end{tabular}
\end{footnotesize}
\end{center}
\end{table}

%%%%%%%%%%%%% TTE every 5 pts

\begin{table}
\begin{center}
\begin{footnotesize}
\caption{Single-arm trials with survival outcomes, with interim analyses conducted every 5 patients: pFDR, FDR, bias, MSE,  coverage of posterior credible intervals, and ATIE, evaluated with or without interim stopping, under various user-specified priors with $\theta_0=8$ and data-generating prior $\pi_g(\theta)=\mbox{Gamma}(12,2)$ and $\pi_g(\kappa)=\mbox{Gamma}(8,2)$.}
\begin{tabular}{lccccccc}
\hline
\hline

$\pi(\theta)$ &      Interims &        pFDR &     FDR &     Bias  ($\times 10^{-3}$)                    &    MSE & Coverage &       ATIE    \\

              %    &                    &                   &            &   ($\times 10^{-3}$)    &            &         &          \\
\hline

$\theta\sim\mbox{Gamma}(128,16)$ &         no &      0.072&0.009&166.473&0.121&0.739&0.010 \\

$\kappa\sim\mbox{Gamma}(32,8)$ &        yes &      0.280&0.048&125.012&0.307&0.710&0.055 \\

           &            &            &            &            &            &            &                   \\

$\theta\sim\mbox{Gamma}(21.33, 2.67)$ &         no &     0.061&0.007&36.043&0.051&0.942&0.008\\

$\kappa\sim\mbox{Gamma}(8, 2)$ &        yes &      0.397&0.082&132.023&0.357&0.931&0.094\\

           &            &            &            &            &            &            &                   \\

$\theta\sim\mbox{Gamma}(0.64, 0.08)$ &         no &      0.058&0.007&-0.621&0.051&0.948&0.008\\

$\kappa\sim\mbox{Gamma}(0.16, 0.04)$ &        yes &      0.718&0.322&3239.102&32.548&0.891&0.370\\

           &            &            &            &            &            &            &                   \\

$\theta\sim\mbox{Gamma}(72, 12)$ &         no &     0.017&0.002&-15.771&0.072&0.892&0.002\\

$\kappa\sim\mbox{Gamma}(32,8)$ &        yes &  0.035&0.004&-83.678&0.238&0.863&0.004\\

             &            &            &            &            &            &            &                   \\

$\theta\sim\mbox{Gamma}(12, 2)^*$ &         no &     0.050&0.006&-1.641&0.049&0.949&0.007\\

$\kappa\sim\mbox{Gamma}(8, 2)^*$ &        yes &     0.221&0.034&-7.936&0.188&0.946&0.039\\

             &            &            &            &            &            &            &                   \\

$\theta\sim\mbox{Gamma}(0.36, 0.06)$ &         no &     0.059&0.007&-1.792&0.051&0.949&0.008\\

$\kappa\sim\mbox{Gamma}(0.16, 0.04)$ &        yes &     0.713&0.314&3466.480&39.635&0.894&0.360 \\

             &            &            &            &            &            &            &                   \\
$\theta\sim\mbox{Gamma}(200, 20)$ &         no &       0.235&0.038&428.380&0.362&0.420&0.043\\

$\kappa\sim\mbox{Gamma}(32, 8)$ &        yes &      0.872&0.872&3755.907&16.813&0.073&1.000\\

             &            &            &            &            &            &            &                   \\

$\theta\sim\mbox{Gamma}(33.33, 3.33)$ &         no &     0.082&0.010&91.852&0.064&0.914&0.012\\

$\kappa\sim\mbox{Gamma}(8, 2)$ &        yes &      0.846&0.703&2594.147&10.015&0.464&0.807 \\

               &            &            &            &            &            &            &                   \\

$\theta\sim\mbox{Gamma}(1, 0.1)$ &         no &      0.059&0.007&1.228&0.051&0.949&0.008 \\

$\kappa\sim\mbox{Gamma}(0.16, 0.04)$ &        yes &     0.736&0.352&3373.016&31.409&0.883&0.403\\

\hline
\hline
\end{tabular}
\end{footnotesize}
\end{center}
\end{table}

\begin{table}
\begin{center}
\begin{footnotesize}
\caption{Single-arm trials with normal outcomes with a known variance of 1: pFDR, FDR, bias, MSE,  coverage of posterior credible intervals, and ATIE, evaluated with or without interim stopping, under various user-specified priors with $\theta_0=0.25$ and data-generating prior is $\pi_g(\theta) = N(0,0.09)$. }
\begin{tabular}{lccccccc}
\hline
\hline

$\pi(\theta)$ &      Interims &        pFDR &     FDR &     Bias  ($\times 10^{-3}$)                    &    MSE & Coverage &      ATIE  \\

 %                 &                    &                   &            &   ($\times 10^{-3}$)    &            &         &           \\
\hline

N(0.25, 0.03) &         no &     0.064&0.009&62.805&0.015&0.827&0.011\\

           &        yes &      0.122&0.019&61.555&0.017&0.824&0.024 \\

               &            &            &            &            &            &            &                   \\

N(0.25, 0.09) &         no &      0.074&0.010&25.219&0.010&0.942&0.013 \\

           &        yes &      0.144&0.024&28.953&0.011&0.940&0.030 \\

              &            &            &            &            &            &            &                   \\

N(0.25, 1000) &         no &      0.079&0.011&0.165&0.010&0.950&0.014 \\

           &        yes &      0.158&0.028&9.966&0.013&0.945&0.035 \\

               &            &            &            &            &            &            &                   \\

N(0, 0.03) &         no &      0.015&0.001&0.305&0.011&0.888&0.002 \\

           &        yes &      0.023&0.002&-3.067&0.013&0.882&0.003 \\

              &            &            &            &            &            &            &                   \\

N(0, 0.09) &         no &      0.050&0.006&0.219&0.009&0.949&0.008 \\

           &        yes &      0.090&0.013&0.186&0.010&0.950&0.016 \\

               &            &            &            &            &            &            &                   \\

N(0, 1000) &         no &      0.079&0.011&0.163&0.010&0.950&0.014 \\

           &        yes &      0.158&0.028&9.963&0.013&0.945&0.035 \\

               &            &            &            &            &            &            &                   \\

N(0.5, 0.03) &         no &      0.172&0.034&125.305&0.027&0.660&0.043 \\

           &        yes &     0.350&0.099&139.836&0.033&0.638&0.124\\

               &            &            &            &            &            &            &                   \\

N(0.5, 0.09) &         no &      0.102&0.016&50.219&0.012&0.917&0.020 \\

           &        yes &      0.210&0.043&60.118&0.015&0.909&0.054 \\

               &            &            &            &            &            &            &                   \\
               
N(0.5, 1000) &         no &     0.079&0.011&0.168&0.010&0.950&0.014 \\

           &        yes &      0.158&0.028&9.969&0.013&0.945&0.035\\

\hline
\hline
\end{tabular}
\end{footnotesize}
\end{center}
\end{table}

\begin{table}
\begin{center}
\begin{footnotesize}
\caption{Single-arm trials with binary outcomes: pFDR, FDR, bias, MSE,  coverage of posterior credible intervals, and ATIE,  evaluated with or without interim stopping, under various user-specified priors with $\theta_0=0.6$ and data-generating prior $\pi_g(\theta) = \mbox{Beta}(15,15)$. }
\begin{tabular}{lccccccc}
\hline
\hline

$\pi(\theta)$ &      Interims &        pFDR &     FDR &     Bias  ($\times 10^{-3}$)                    &    MSE & Coverage &      ATIE     \\

 %                 &                    &                   &            &   ($\times 10^{-3}$)    &            &         &           \\
\hline

Beta(36, 24) &         no &      0.094&0.004&37.754&0.003&0.795&0.005 \\

           &        yes &      0.121&0.006&37.836&0.004&0.794&0.007 \\

                     &            &            &            &            &            &            &                   \\

Beta(18, 12) &         no &      0.094&0.004&23.294&0.002&0.918&0.005 \\

           &        yes &      0.151&0.008&23.838&0.002&0.917&0.010 \\

                      &            &            &            &            &            &            &                   \\

Beta(0.06, 0.04) &         no &      0.120&0.007&0.257&0.002&0.950&0.008 \\

           &        yes &      0.260&0.022&3.905&0.003&0.943&0.025\\

                      &            &            &            &            &            &            &                   \\

Beta(30, 30) &         no &     0.016&0.000&0.254&0.002&0.907&0.000 \\

           &        yes &     0.016&0.000&0.235&0.002&0.907&0.000 \\

                      &            &            &            &            &            &            &                   \\

Beta(15, 15) &         no &      0.045&0.001&0.217&0.002&0.950&0.001\\

           &        yes &      0.063&0.002&0.230&0.002&0.950&0.002 \\

                      &            &            &            &            &            &            &                   \\

Beta(0.05, 0.05) &         no &      0.120&0.007&0.157&0.002&0.950&0.008 \\

           &        yes &     0.260&0.022&3.796&0.003&0.943&0.025 \\

                      &            &            &            &            &            &            &                   \\

Beta(42, 18) &         no &      0.319&0.042&75.254&0.008&0.510&0.048 \\

           &        yes &      0.508&0.109&81.571&0.009&0.483&0.125\\

                      &            &            &            &            &            &            &                   \\

Beta(21, 9) &         no &     0.189&0.015&46.370&0.004&0.816&0.017\\

           &        yes &     0.349&0.043&50.153&0.005&0.803&0.050 \\

                      &            &            &            &            &            &            &                   \\

Beta(0.07, 0.03) &         no &      0.120&0.007&0.357&0.002&0.950&0.008 \\

           &        yes &      0.260&0.022&4.014&0.003&0.943&0.025 \\

\hline
\hline
\end{tabular}
\end{footnotesize}
\end{center}
\end{table}
%%%%%%%%%%%%%%%%%%%%%%%TTE pr(H0) -- cutoff = 0.74 %%%%%%%%%%%%%
\begin{table}
\begin{center}
\begin{footnotesize}
\caption{Single-arm trials with time-to-event outcomes: pFDR, FDR, bias, MSE,  coverage of posterior credible intervals, and ATIE,  evaluated with or without interim stopping, under various user-specified priors with $\theta_0=6$ and data-generating prior $\mbox{Gamma}(24,4)$ for $\theta$ and $\mbox{Gamma}(8,2)$ for $\kappa$. }

\begin{tabular}{lccccccc}
\hline
\hline

$\pi(\theta)$ &      Interims &        pFDR &     FDR &     Bias  ($\times 10^{-3}$)                    &    MSE & Coverage &      ATIE    \\

 %                 &                    &                   &            &   ($\times 10^{-3}$)    &            &         &           \\
\hline

$\theta\sim\mbox{Gamma}(640, 80)$ &         no &      0.070&0.003&643.976&0.747&0.218&0.004 \\

$\kappa\sim\mbox{Gamma}(32,8)$ &        yes &      0.106&0.005&637.294&0.759&0.215&0.006 \\

            &            &            &            &            &            &            &                   \\

$\theta\sim\mbox{Gamma}(42.67, 5.33)$ &         no &      0.075&0.004&72.468&0.055&0.925&0.004 \\

$\kappa\sim\mbox{Gamma}(8, 2)$ &        yes &    0.201&0.012&82.889&0.074&0.924&0.013 \\

        &            &            &            &            &            &            &                   \\

$\theta\sim\mbox{Gamma}(0.64, 0.08)$ &         no &      0.074&0.004&-1.296&0.049&0.948&0.004 \\

$\kappa\sim\mbox{Gamma}(0.16, 0.04)$ &        yes &      0.471&0.046&361.649&3.018&0.935&0.049 \\

            &            &            &            &            &            &            &                   \\

$\theta\sim\mbox{Gamma}(360, 60)$ &         no &      0.000&0.000&-51.030&0.187&0.637&0.000\\

$\kappa\sim\mbox{Gamma}(32,8)$ &        yes &      0.000&0.000&-51.030&0.187&0.637&0.000 \\

           &            &            &            &            &            &            &                   \\

$\theta\sim\mbox{Gamma}(24, 4)$ &         no &      0.050&0.002&-2.132&0.046&0.949&0.002 \\

$\kappa\sim\mbox{Gamma}(8, 2)$ &        yes &      0.097&0.005&-2.233&0.053&0.949&0.005 \\

        &            &            &            &            &            &            &                   \\
$\theta\sim\mbox{Gamma}(0.36, 0.06)$ &         no &      0.074&0.004&-2.506&0.049&0.948&0.004 \\

$\kappa\sim\mbox{Gamma}(0.16, 0.04)$ &        yes &      0.465&0.045&388.648&3.844&0.934&0.047 \\

     &            &            &            &            &            &            &                   \\

$\theta\sim\mbox{Gamma}(1000, 100)$ &         no &     0.886&0.466&2199.969&6.379&0.016&0.496\\

$\kappa\sim\mbox{Gamma}(32, 8)$ &        yes &      0.940&0.940&3820.645&15.991&0.007&1.000 \\

     &            &            &            &            &            &            &                   \\

$\theta\sim\mbox{Gamma}(66.67, 6.67)$ &         no &      0.146&0.009&179.058&0.101&0.833&0.009\\

$\kappa\sim\mbox{Gamma}(8, 2)$ &        yes &      0.858&0.356&1113.670&3.008&0.598&0.379 \\

     &            &            &            &            &            &            &                   \\

$\theta\sim\mbox{Gamma}(1, 0.1)$ &         no &      0.075&0.004&0.561&0.049&0.949&0.004\\

$\kappa\sim\mbox{Gamma}(0.16, 0.04)$ &        yes &      0.486&0.049&376.358&2.910&0.933&0.052 \\

\hline
\hline
\end{tabular}
\end{footnotesize}
\end{center}
\end{table}

\begin{table}
\begin{center}
\begin{footnotesize}
\caption{Single-arm trials with normal outcomes with an unknown variance: pFDR, FDR, bias, MSE,  coverage of posterior credible intervals, and ATIE, evaluated with or without interim stopping, under various user-specified priors, when the scale parameter $\sigma_U^2=20$ for the user-specified prior with $\theta_0=0$ and data-generating prior $\pi_g(\theta|\sigma^2)= N(0,\sigma^2/5)$ and $\pi_g(\sigma^2)= \mbox{Inv-}\chi^2(5,40)$. }
\begin{tabular}{lccccccc}
\hline
\hline

$\pi(\theta)$ &      Interims &        pFDR &     FDR &     Bias  ($\times 10^{-3}$)                    &    MSE & Coverage &     ATIE     \\

 %                 &                    &                   &            &   ($\times 10^{-3}$)    &            &         &           \\
\hline

$\theta|\sigma^2\sim N(0.25,\sigma^2/20)$ &         no &      0.051&0.022&39.360&0.837&0.881&0.042 \\

$\sigma^2\sim Inv-\chi^2(20,20)$ &        yes &      0.097&0.047&-103.279&1.468&0.850&0.088 \\

         &            &            &            &            &            &            &                   \\

$\theta|\sigma^2\sim N(0.25,\sigma^2/5)$ &         no &    0.052&0.023&11.550&0.633&0.948&0.043 \\

$\sigma^2\sim Inv-\chi^2(5,20)$ &        yes &      0.100&0.048&15.431&1.017&0.945&0.091 \\

          &            &            &            &            &            &            &                   \\

$\theta|\sigma^2\sim N(0.25,\sigma^2/0.1)$ &         no &      0.052&0.023&0.659&0.664&0.950&0.043 \\

$\sigma^2\sim Inv-\chi^2(0.1,20)$ &        yes &      0.100&0.049&90.452&1.119&0.949&0.092 \\

          &            &            &            &            &            &            &                   \\

$\theta|\sigma^2\sim N(0,\sigma^2/20)$ &         no &      0.047&0.020&-2.307&0.836&0.881&0.038\\

$\sigma^2\sim Inv-\chi^2(20,20)$ &        yes &     0.086&0.041&-162.353&1.496&0.848&0.076 \\

           &            &            &            &            &            &            &                   \\

$\theta|\sigma^2\sim N(0,\sigma^2/5)$ &         no &     0.050&0.022&-0.355&0.633&0.948&0.042 \\

$\sigma^2\sim Inv-\chi^2(5,20)$ &        yes &      0.096&0.046&-3.468&1.014&0.946&0.087 \\

           &            &            &            &            &            &            &                   \\
$\theta|\sigma^2\sim N(0,\sigma^2/0.1)$ &         no &     0.052&0.023&0.409&0.664&0.950&0.043 \\

$\sigma^2\sim Inv-\chi^2(0.1,20)$ &        yes &     0.100&0.049&90.033&1.119&0.949&0.092\\

           &            &            &            &            &            &            &                   \\
$\theta|\sigma^2\sim N(0.5,\sigma^2/20)$ &         no &     0.056&0.025&81.027&0.842&0.879&0.047 \\

$\sigma^2\sim Inv-\chi^2(20,20)$ &        yes &    0.109&0.054&-43.075&1.449&0.849&0.101 \\

          &            &            &            &            &            &            &                   \\

$\theta|\sigma^2\sim N(0.5,\sigma^2/5)$ &         no &      0.053&0.024&23.454&0.634&0.947&0.044 \\

$\sigma^2\sim Inv-\chi^2(5,20)$ &        yes &     0.103&0.050&34.560&1.020&0.945&0.094\\

           &            &            &            &            &            &            &                   \\

$\theta|\sigma^2\sim N(0.5,\sigma^2/0.1)$ &         no &      0.052&0.023&0.908&0.664&0.950&0.043\\

$\sigma^2\sim Inv-\chi^2(0.1,20)$ &        yes &     0.100&0.049&90.883&1.119&0.949&0.092 \\

\hline
\hline
\end{tabular}
\end{footnotesize}
\end{center}
\end{table}
%%%%%%%%%%%%%%%%%%%%%%%%
\begin{table}
\begin{center}
\begin{footnotesize}
\caption{Single-arm trials with normal outcomes with an unknown variance: pFDR, FDR, bias, MSE,  coverage of posterior credible intervals, and ATIE, evaluated with or without interim stopping, under various user-specified priors, when the scale parameter $\sigma_U^2=60$ for the user-specified prior with $\theta_0=0$ and data-generating prior $\pi_g(\theta|\sigma^2)= N(0,\sigma^2/5)$ and $\pi_g(\sigma^2)= \mbox{Inv-}\chi^2(5,40)$. }
\begin{tabular}{lccccccc}
\hline
\hline

$\pi(\theta)$ &      Interims &        pFDR &     FDR &     Bias  ($\times 10^{-3}$)                    &    MSE & Coverage &      ATIE     \\

 %                 &                    &                   &            &   ($\times 10^{-3}$)    &            &         &           \\
\hline

$\theta|\sigma^2\sim N(0.25,\sigma^2/20)$ &         no &     0.049&0.021&39.360&0.837&0.907&0.040 \\

$\sigma^2\sim Inv-\chi^2(20,60)$ &        yes &      0.091&0.043&-103.534&1.463&0.891&0.082 \\

              &            &            &            &            &            &            &                   \\

$\theta|\sigma^2\sim N(0.25,\sigma^2/5)$ &         no &      0.051&0.023&11.550&0.633&0.953&0.042\\

$\sigma^2\sim Inv-\chi^2(5,60)$ &        yes &      0.098&0.047&15.367&1.016&0.954&0.089\\

              &            &            &            &            &            &            &                   \\

$\theta|\sigma^2\sim N(0.25,\sigma^2/0.1)$ &         no &      0.052&0.023&0.659&0.664&0.950&0.043 \\

$\sigma^2\sim Inv-\chi^2(0.1,60)$ &        yes &    0.100&0.049&90.447&1.119&0.949&0.092 \\

              &            &            &            &            &            &            &                   \\

$\theta|\sigma^2\sim N(0,\sigma^2/20)$ &         no &     0.045&0.020&-2.307&0.836&0.908&0.037 \\

$\sigma^2\sim Inv-\chi^2(20,60)$ &        yes &      0.082&0.038&-161.389&1.492&0.889&0.072 \\

              &            &            &            &            &            &            &                   \\

$\theta|\sigma^2\sim N(0,\sigma^2/5)$ &         no &      0.050&0.022&-0.355&0.633&0.953&0.041\\

$\sigma^2\sim Inv-\chi^2(5,60)$ &        yes &      0.095&0.045&-3.697&1.012&0.954&0.086\\

              &            &            &            &            &            &            &                   \\

$\theta|\sigma^2\sim N(0,\sigma^2/0.1)$ &         no &      0.052&0.023&0.409&0.664&0.950&0.043 \\

$\sigma^2\sim Inv-\chi^2(0.1,60)$ &        yes &      0.100&0.049&90.040&1.119&0.949&0.092 \\

              &            &            &            &            &            &            &                   \\

$\theta|\sigma^2\sim N(0.5,\sigma^2/20)$ &         no &      0.054&0.024&81.027&0.842&0.906&0.045 \\

$\sigma^2\sim Inv-\chi^2(20,60)$ &        yes &      0.103&0.050&-43.282&1.445&0.891&0.094 \\

              &            &            &            &            &            &            &                   \\

$\theta|\sigma^2\sim N(0.5,\sigma^2/5)$ &         no &      0.052&0.023&23.454&0.634&0.953&0.044 \\

$\sigma^2\sim Inv-\chi^2(5,60)$ &        yes &      0.101&0.049&34.456&1.019&0.954&0.092\\

              &            &            &            &            &            &            &                   \\

$\theta|\sigma^2\sim N(0.5,\sigma^2/0.1)$ &         no &      0.052&0.023&0.908&0.664&0.950&0.043 \\

$\sigma^2\sim Inv-\chi^2(0.1,60)$ &        yes &     0.100&0.049&90.829&1.119&0.949&0.092 \\

\hline
\hline
\end{tabular}
\end{footnotesize}
\end{center}
\end{table}

\end{document}
